# Supplementary material for: 3D Paintbrush: Local Stylization of 3D Shapes with Cascaded Score Distillation
Source: arXiv:2311.09571 source file (2023-11-16)
Supplement: Supplementary file 1 [file X_suppl.tex]

\clearpage
\setcounter{page}{1}
\maketitlesupplementary
